# Supplementary material for: Learning Object Detection from Captions via Textual Scene Attributes
Source: arXiv:2009.14558 source file (2020-09-30)
Supplement: Supplementary file 1 [file supp.tex]

\newpage
\setcounter{section}{0} %% Start counting from the beginning

In this supplementary file we provide additional implementation details, and empirical results. 
\section{bla} 
\label{sec:bla}
